# Supplementary material for: A Tight Approximation for Submodular Maximization with Mixed Packing and Covering Constraints
Source: arXiv:1804.10947 source file (2018-12-19)
Supplement: Supplementary file 2 [file OneSidedFeasible-Algorithm-Appendix-old.tex]

Below, we give a full technical description of the proof of our main Theorem~\ref{thrm:MainApproximation}. We refer to Our Techniques in Section~\ref{sec:Introduction} and Section~\ref{sec:multi-linear-relaxation} for a comprehensive intuitive exposition.

\subsection{Algorithm}
\label{apx-subsec:one-sided-algo}
Let $b=c+p$ be the total number of constraints. Let $\alpha, \beta, \gamma, \delta \in (0, 1)$ be some parameters, which we fix later.
\noindent Recall that $O$ denotes some fixed optimal solution for \PCSM (\ref{Objective}).

We define a {\em guess} $D$ to be a triplet $(E_0,E_1,\mathbf{c}')$, where $E_0\subseteq \mathcal{N}$ denotes elements that are discarded, $E_1\subseteq \mathcal{N}$ denotes elements that are chosen, and $\mathbf{c}'\in \mathbb{R}_+^c$ represents a rough estimate (up to a factor of $1+\varepsilon$) of how much an optimal solution $O$ covers each of the covering constraints, {\em i.e.}, $\mathbf{C} \mathbf{1}_O$.
Let us denote by $\tilde{\mathcal{N}} \triangleq \mathcal{N} \setminus (E_0\cup E_1)$ the remaining undetermined elements with respect to guess $D$.

Given any guess $D$, we define the {\em residual} objective and constraints.

First, we define the residual objective $g^D:2^{\cN\setminus \left( E_0\cup E_1\right)}\rightarrow\R_+$ by:
\[g^D(T)\triangleq f(T\cup E_1) - f(E_1)~~~~~~~\forall T\subseteq \cN\setminus \left( E_0\cup E_1\right).\]

As in Section~\ref{sec:multi-linear-relaxation}, $g^D$ is monotone, submodular, and non-negative since the original set function $f$ is monotone non-decreasing.
Second, let us focus on the residual constraints.
Denote by $\bP_{\cN\setminus (E_0\cup E_1)}$ the sub-matrix of $\bP$ obtained by choosing all the columns in $\cN\setminus (E_0\cup E_1)$.
Consider $\rd \in \R_+^p$, the residual value that can still be packed by the algorithm with respect to the $i^{\text{th}}$ packing constraint: \[ \rdi \triangleq 1 -\sum _{\ell\in E_1}\bP_{i,\ell}~~~~~~~\forall i \in [p].\]


Consider $\sd \in \R_+^c$, the residual value that still needs to be covered by the algorithm with respect to the $j^{\text{th}}$ covering constraint: \[ \sdj \triangleq \max\left\{0, \bc'_j-\sum _{\ell\in E_1}\bC_{j,\ell}\right\}~~~~~~~\forall j \in [c].\]
Note that $\zero_c \leq \sd$, where $\zero_k \triangleq 0 \cdot \one_k$ for any $\one_k \in \R^k$.

For any guess $D=(E_0,E_1, \bc')$, the residual problem that needs to be solved is:
\begin{align}
\max\left\{ f(E_1)+g^D(T):T\subseteq \cN\setminus (E_0\cup E_1), \bP_{\cN\setminus (E_0\cup E_1)}\mathbf{1}_S\leq \rd, \bC_{\cN\setminus (E_0\cup E_1)}\mathbf{1}_S\geq \sd \right\}.\label{apx-OneSidedObjectiveResidual}
\end{align}

We define the following two polytopes:
\begin{align*}
\cP^D & \triangleq \left\{ \bx\in [0,1]^{\cN\setminus (E_0\cup E_1)}:\bP_{\cN\setminus (E_0\cup E_1)} \bx \leq \rd \right\}\\
\cC^D & \triangleq \left\{ \bx \in [0,1]^{\cN\setminus (E_0\cup E_1)}:\bC_{\cN\setminus (E_0\cup E_1)}\bx \geq \sd \right\}.
\end{align*}

Furthermore, denote by $G^D:[0,1]^{\cN\setminus (E_0\cup E_1)}\rightarrow \R_+$ the multilinear extension of $g^D$.
Hence, the continuous multilinear relaxation of (\ref{apx-OneSidedObjectiveResidual}) is the following:
\begin{align}
\max\left\{ f(E_1)+G^D(\bx):\bx\in [0,1]^{\cN\setminus (E_0\cup E_1)}, \bx \in \cP^D\cap \cC^D\right\}.\label{apx-ObjectiveContinuous}
\end{align}

%The continuous greedy algorithm receives a ground set $\cN$, a continuous function to maximize $F$ and a polytope $P$.
%in polynomial time, the continuous greedy algorithm finds a fractional point $X^* \in P$ such that $F(X^*) \geq (1-\frac{1}{\e})\opt$ for some optimal integral solution $O$.


A packing constraint $i \in [p]$ (or a covering constraint $j \in [c]$) is called \emph{critical} constraint if $\rdi \leq \delta$ (or $\sdj \leq \delta  \bc'_j$). Below we define sets of constraint which are critical.
\[Y_D \triangleq \left\{ i =1, \dots, p : \rdi \leq \delta \right\};~~~~~~~ Z_D \triangleq \left\{ j=1,\dots,c: \sdj \leq \delta \bc'_j \right\} \]

The sets $P_D, C_D$ will be the set of elements which are \emph{large} with respect to the residual value of some non-critical packing, covering constraint respectively.
\[P_D \triangleq \left\{ \ell \in \residual: \exists i \in ([p] \setminus Y_D) \, \bP_{i, \ell} \geq \alpha \cdot \rdi \right\} \]
\[C_D \triangleq \left\{ \ell \in \residual: \exists j \in ([c] \setminus Z_D) \, \bC_{j, \ell} \geq \alpha \cdot \sdj \right\} \]


We also define below the set  $L_D$ of elements which are large with respect to critical packing constraints.
\[L_D \triangleq \left\{ \ell \in \residual: \exists i \in  Y_D \,~~ \bP_{i, \ell} \geq \beta \cdot \rdi \right\} \]

The following definition states when a guess $D$ is \emph{consistent}.

\begin{defn}\label{apx-def:OneSidedConsistentGuess}
	A guess $D=(E_0,E_1, \bc')$ is {\em consistent} if:
	\begin{enumerate}
		\item\label{apx-item:oneSidedConsistentDisjoint} $E_0\cap E_1 = \varnothing$.
		\item\label{apx-item:oneSidedConsistentGuessCover}   $\bc'\geq\one_c$.
		%\item $\bC_{j,\ell} <\alpha \bc'_j$  for every covering constraint $j \in [c]$ and every $\ell \in \residual$.
		\item\label{apx-item:oneSidedConsistentGuessPack} $\bP\one_{E_1} \leq \one_p$.
		\item\label{apx-item:oneSidedConsistentGuessNoBig} $P_D = C_D = \varnothing$.
		%\item\label{apx-item:oneSidedConsistentGuessMarginal} For any $\ell \in \residual$, $f_{E_1}(\ell) \leq \gamma^{-1}f(E_1)$.
		%\item $\mathbf{0}_p \leq \rd$
		%\item $\bP_{i,\ell}<\alpha$ for every packing constraint $i \in [p]$ and every $\ell \in \residual$.
	\end{enumerate}
\end{defn}

Now we produces a list of consistent guesses that contains at least one guess that is \emph{correct} (see Definition~\ref{apx-def:OneSidedCorrectGuess}) with respect to the optimal solution $O$.
%Our preprocessing step produces a consistent guess which is also correct with respect to some optimal solution $S^*$.
%Since the algorithm cannot verify whether a consistent guess is also correct, it produces a list of consistent guesses that contains at least one guess that is correct.
%We now are ready to formally define our preprocessing algorithm.

\begin{algorithm*}[H] \label{apx-alg:OneSidedGuessesEnumeration}
	\caption{Preprocessing}
	$\cL \leftarrow \varnothing$ \\
	%Enumerate over $Z \subseteq \{1,...,c\}$.
	\ForEach{$j_1,\dots,j_c\in\{0,1,\dots,\lceil\log_{1+\delta} n\rceil\}$}{
		Let $\bc' = ((1+\delta)^{j_1},\dots,(1+\delta)^{j_c})$\\
		 %Enumerate over all set $E_1 . \\
		\ForEach{$E_1\subseteq \cN$ such that $|E_1| \leq \gamma + \nicefrac{(p+c)}{(\alpha \delta)}$}{
			Let $H = (\varnothing, E_1, \bc')$\\
			Let $E_0 = \{\ell \in \cN \setminus E_1: f_{E_1}(\ell) > (\gamma^{-1}) f(E_1)\} \cup P_H \cup C_H$\label{apx-alg:E_0}\\
		        Set $D=(E_0, E_1, \bc')$\\
		        If $D$ is consistent according to Definition \ref{Definition:consistent} add it to $\cL$.
		}
	}
	Output $\cL$.
\end{algorithm*}

Now we define our main algorithm.

\begin{algorithm*}[H]
	\caption{$(f,\cN,\bP,\bC)$}\label{apx-alg:OneSidedMainAlgorithm}
	Use Algorithm \ref{apx-alg:OneSidedGuessesEnumeration} to obtain a list of guesses $\cL$. \\
	\ForEach{$D=(E_0, E_1,\bc') \in \cL$}{
          Use Theorem~\ref{thrm:ContGreedy} to compute an approximate solution $\bx^*$ to problem (\ref{apx-ObjectiveContinuous}).\label{apx-alg:OneSidedMainAlgorithm-ContGreedy}\\
		Scale down $\x^*$ to $\bar{\x} = \x^*/(1+\delta)$\\
		Let $R_D$ be such that for every $\ell \in \tilde{\mathcal{N}}$ independently: $\Pr \left[ \ell \in R_D\right] = \bar{\x}_{\ell}$.\\
		Let $R'_D = R_D \setminus L_D$.\\
		$S_D \leftarrow E_1 \cup R'_D$.
		}
	$S_{alg} \leftarrow \argmax \left\{f(S_D) : D\in \cL, \bP \cdot \one_{S_D} \leq \one_p, \bC \cdot \one_{S_D} \geq (1-\eps)\one _c \right\}$
	%Output: $E_1 \cup R'_D$ of max objective value, such that $\bP\cdot \one_{E_1 \cup R'_D} \leq \one, \bC \cdot \one_{E_1 \cup R'_D} \geq (1-\eps)\one$
\end{algorithm*}
%\begin{itemize}
  %  \item By exploring all vectors $\bC \times ((1+\eps)^{j_1},\dots,(1+\eps)^{j_d})$, for $j_1,\dots,j_d\in\{0,1,\dots,\lceil\log_{1+\eps} n\rceil\}$ we guess a profit vector $\bC^*$ that satisfies $\bC\leq \bC^* \leq p(O)\leq(1+\eps)\bC^*$. From now on we assume $\bC$ to be equal to $\bC^*$.
 %   \item Enumerate all sets $A$ of size at most $(b+1)/\eps^9$.\sumi{Optimize this parameter.} (We are guessing the most valuable elements and large elements in the optimum solution.) For each candidate set $A$ repeat the following.
%    \item Let $\bP'=\bP-\sum_{e\in A}\w_e$ and $\bc'=\bC-\sum_{e\in A}\p_e$ be the residual weight and profit vector, respectively.
%    \begin{itemize}
 %   	\item If some entry in $\bP'$ is negative continue with the next guess for~$A$.
%	\item Set all negative entries in $\bc'$ to $0$.
 %   \end{itemize}
%    \item Let $B$ be the set of elements $e$ that satisfy $f_A(e)>\eps^4f(A)$ or that are large with respect to $\bc', \bP'$.
 %   \item We consider a reduced problem on the set $\cN'=\cN\setminus (A\cup B)$, with the residual packing and covering constraints, and with the objective function $g(S)=f_A(S)$. Solve the following optimization problem where $G(x)$ is the multi-linear relaxation of $g$
%    \begin{displaymath}
%    \max\left\{\,G(\mathbf{x})\,\middle|\, \mathbf{x}\in[0,1]^{\cN'}, \sum_{e\in \cN'}\w_e x_e\leq \bP',\sum_{e\in \cN'}\p_e x_e\geq \bc'\,\right\}
%    \end{displaymath}
%    and find a $(1-1/\e)$-approximate solution $\mathbf{x}^*$ for it using the continuous greedy algorithm.
%    \item Scale down $\mathbf{x}^*$ to $\mathbf{x}^*/(1+\eps)$
%    \item Given $\mathbf{x}^*$ use randomized independent rounding to round $\mathbf{x}^*$ to an integral solution $R_A$.
%    \item For all tiny weight constraints $\bP_i'$ remove from $R_A$ all elements $e$ with weight ${w_i(e)\geq\eps^3 \bP_i'}$. Let $R_A'$ be the resulting set.
%    \item Among all solutions guesses for $A$ such that $A\cup R_A'$ is an $\eps$-nearly feasible output one maximizing $f(A\cup R_A')$.
%    \end{itemize}



%%% Local Variables:
%%% mode: latex
%%% TeX-master: "../MainCombined"
%%% End:
